# Supplementary material for: Rigorous Error Analysis for Logarithmic Number Systems
Source: arXiv:2401.17184 source file (2024-01-30)
Supplement: Supplementary file 1 [file appendix2.tex]

\begin{table}[]
\begin{tabular}{|l|l|llllllll|}
\hline
                                     & $\Delta$ &$ 2^{-3}$       & $2^{-4}$       &$ 2^{-5}$       &$ 2^{-6}$       &$ 2^{-7}$       &$ 2^{-8}$       &$ 2^{-9}$       &$ 2^{-10}$      \\ \hline
\multirow{3}{*}{$\Phi^+$}              & Taylor &$ 1.35x10^{-3}$ &$ 3.39x10^{-4}$ &$ 8.47x10^{-5}$ &$ 2.13x10^{-5}$ &$ 5.41x10^{-6}$ &$ 1.44x10^{-6}$ &$ 4.50x10^{-7}$ &$ 2.01x10^{-7}$ \\
                                     & EC1    &$ 1.68x10^{-4}$ &$ 4.17x10^{-5}$ &$ 1.05x10^{-5}$ &$ 2.81x10^{-6}$ &$ 8.80x10^{-7}$ &$ 3.99x10^{-7}$ &$ 2.79x10^{-7}$ &$ 2.48x10^{-7}$ \\
                                     & EC2    &$ 1.63x10^{-5}$ &$ 3.57x10^{-6}$ &$ 9.87x10^{-7}$ &$ 4.15x10^{-7}$ &$ 2.81x10^{-7}$ &$ 2.49x10^{-7}$ &$ 2.41x10^{-7}$ &$ 2.39x10^{-7}$ \\ \hline
\multirow{3}{*}{$\Phi^- (-\infty,-1]$} & Taylor &$ 9.97x10^{-3}$ &$ 2.6x10^{-3}$  &$ 6.63x10^{-4}$ &$ 1.68x10^{-4}$ &$ 4.22x10^{-5}$ &$ 1.07x10^{-6}$ &$ 2.76x10^{-6}$ &$ 7.80x10^{-7}$ \\
                                     & EC1    &$ 1.27x10^{-3}$ &$ 3.23x10^{-4}$ &$ 8.16x10^{-5}$ &$ 2.07x10^{-5}$ &$ 5.35x10^{-6}$ &$ 1.52x10^{-6}$ &$ 5.59x10^{-7}$ &$ 3.19x10^{-7}$ \\
                                     & EC2    &$ 1.54x10^{-4}$ &$ 3.09x10^{-5}$ &$ 6.77x10^{-6}$ &$ 1.72x10^{-6}$ &$ 5.89x10^{-7}$ &$ 3.24x10^{-7}$ &$ 2.59x10^{-7}$ &$ 2.44x10^{-7}$ \\ \hline
\multirow{3}{*}{$\Phi^-$ Cotrans}      & Taylor &$ 2.96x10^{-2}$ &$ 7.77x10^{-3}$  &$ 1.99x10^{-3}$ &$ 5.03x10^{-4}$ &$ 1.27x10^{-4}$ &$ 3.25x10^{-5}$ &$ 8.82x10^{-6}$ &$ 2.88x10^{-6}$ \\
                                     &EC1    &$ 3.8x10^{-3}$ &$ 9.69x10^{-4}$ &$ 2.45x10^{-4}$  &$ 6.25x10^{-5}$ &$ 1.66x10^{-5}$ &$ 5.09x10^{-6}$ &$ 2.21x10^{-6}$ &$ 1.49x10^{-6}$ \\
                                     & EC2    &$ 4.63x10^{-4}$ &$ 9.32x10^{-5}$ &$ 2.08x10^{-5}$ &$ 5.69x10^{-6}$ &$ 2.30x10^{-6}$  &$ 1.51x10^{-6}$ &$ 1.31x10^{-6}$ &$ 1.27x10^{-6}$ \\ \hline
\end{tabular}
\caption{Absolute error of LNS fixed-point representation}
\end{table}

\begin{table}[]
\begin{tabular}{|l|l|llllllll|}
\hline
                                     & $\Delta$ &$ 2^{-3}$       & $2^{-4}$       &$ 2^{-5}$       &$ 2^{-6}$       &$ 2^{-7}$       &$ 2^{-8}$       &$ 2^{-9}$       &$ 2^{-10}$      \\ \hline
\multirow{3}{*}{$\Phi^+$}              & Taylor &$ 9.39x10^{-4}$ &$ 2.35x10^{-4}$ &$ 5.87x10^{-5}$ &$ 1.47x10^{-5}$ &$ 3.74x10^{-6}$ &$ 9.99x10^{-7}$ &$ 3.11x10^{-7}$ &$ 1.39x10^{-7}$ \\
                                     & EC1    &$ 1.16x10^{-4}$ &$ 2.89x10^{-5}$ &$ 7.31x10^{-6}$ &$ 1.95x10^{-6}$ &$ 6.10x10^{-7}$ &$ 2.76x10^{-7}$ &$ 1.93x10^{-7}$ &$ 1.72x10^{-7}$ \\
                                     & EC2    &$ 1.13x10^{-5}$ &$ 2.48x10^{-6}$ &$ 6.84x10^{-7}$ &$ 2.88x10^{-7}$ &$ 1.95x10^{-7}$ &$ 1.73x10^{-7}$ &$ 1.67x10^{-7}$ &$ 1.66x10^{-7}$ \\ \hline
\multirow{3}{*}{$\Phi^- (-\infty,-1]$} & Taylor &$ 6.94x10^{-3}$ &$ 1.8x10^{-3}$  &$ 4.59x10^{-4}$ &$ 1.16x10^{-4}$ &$ 2.93x10^{-5}$ &$ 7.39x10^{-6}$ &$ 1.91x10^{-6}$ &$ 5.41x10^{-7}$ \\
                                     & EC1    &$ 8.79x10^{-4}$ &$ 2.24x10^{-4}$ &$ 5.65x10^{-5}$ &$ 1.43x10^{-5}$ &$ 3.71x10^{-6}$ &$ 1.05x10^{-6}$ &$ 3.87x10^{-7}$ &$ 2.21x10^{-7}$ \\
                                     & EC2    &$ 1.07x10^{-4}$ &$ 2.14x10^{-5}$ &$ 4.69x10^{-6}$ &$ 1.19x10^{-6}$ &$ 4.08x10^{-7}$ &$ 2.24x10^{-7}$ &$ 1.80x10^{-7}$ &$ 1.69x10^{-7}$ \\ \hline
\multirow{3}{*}{$\Phi^-$ Cotrans}      & Taylor &$ 2.08x10^{-2}$ &$ 5.4x10^{-3}$  &$ 1.38x10^{-3}$ &$ 3.49x10^{-4}$ &$ 8.81x10^{-5}$ &$ 2.26x10^{-5}$ &$ 6.11x10^{-6}$ &$ 1.99x10^{-6}$ \\
                                     &EC1    &$ 2.63x10^{-3}$ &$ 6.72x10^{-4}$ &$ 1.7x10^{-4}$  &$ 4.33x10^{-5}$ &$ 1.15x10^{-5}$ &$ 3.53x10^{-6}$ &$ 1.53x10^{-6}$ &$ 1.03x10^{-6}$ \\
                                     & EC2    &$ 3.21x10^{-4}$ &$ 6.45x10^{-5}$ &$ 1.44x10^{-5}$ &$ 3.95x10^{-6}$ &$ 1.6x10^{-6}$  &$ 1.04x10^{-6}$ &$ 9.11x10^{-7}$ &$ 8.79x10^{-7}$ \\ \hline
\end{tabular}
\caption{Relative error of LNS in real domain}
\end{table}
